# Supplementary material for: In-context Examples Selection for Machine Translation
Source: arXiv:2212.02437 source file (2022-12-05)
Supplement: Supplementary file 1 [file bloom_exps.tex]

% \begin{table}[h]
% \centering
% \begin{tabular}{lr}
%  \toprule
%  \textbf{Model}  & \textbf{\bleu} \\
%   \midrule
% Bloom-7b & 23.97 \\
% Bloom-135b & \\
% \midrule
% $\text{XGLM}_{7.5B}$  & 32.14 \\
%   \bottomrule
%  \end{tabular}
% \caption{\bleu using different \plm(s).}\label{tab:bloom_exp}
% \end{table}
